# Supplementary material for: Cosmos-Transfer1: Conditional World Generation with Adaptive Multimodal Control
Source: arXiv:2503.14492 source file (2025-04-01)
Supplement: Supplementary file 1 [file spatiotemporal_ablations.tex]

\section{Spatiotemporal ablations}
\label{sec:spatiotemporal_ablations}

\input{figures/overall-spatiotemporal}

In Figure~\ref{fig:overall-spatiotemporal}, we ablate blur and/or canny weights on foreground pixels, and depth and/or segmentation weights on background pixels. 
While a multitude of heuristics could be used, we choose this specific configuration to exemplify a situation in which the user wants to have close resemblance to the original videos for the salient objects in the scene but generate more diverse videos in the background. We can achieve this by using low-degree of freedom blur and canny controls for the foreground, and higher degree of freedom depth and segmentation controls for the background.
Figure~\ref{fig:overall-spatiotemporal} shows that the blur SSIM and canny F1 scores are highly correlated to blur and canny control weights for foreground pixels. Similarly, depth si-RSME is inversely correlated to depth control weights for background pixels.
